# Supplementary material for: A minimal model for excitons within time-dependent density-functional theory
Source: arXiv:1202.4779 ancillary file (2012-02-21)
Supplement: Supplementary file 1 [file supplemental.pdf]

# Supplemental material for "A minimal model for excitons within time-dependent density-functional theory"

Zeng-hui Yang, Yonghui Li, and Carsten A. Ullrich[1]

*Department of Physics and Astronomy, University of Missouri, Columbia, MO 65211*

(Dated: 21 February 2012)

## I. NUMBER OF DISCRETE EIGENVALUES WHEN THE MATRIX HAS A CERTAIN SYMMETRY

Consider a real $(2n+1)\times(2n+1)$ ($n$ is a positive integer) matrix $\Omega^{(0)}+F$, where $\Omega^0$ is a diagonal real matrix with $\Omega^0_{k,k}=\Omega^{(0)}_{-k,-k}=\omega^{(0)}_k$. In other words, the eigenvalues of $\Omega^0$ are doubly degenerate, except for $\omega^{(0)}_0$. $F$ has the symmetry $F_{k,k'}=F_{-k',-k}=F_{k',k}=F_{-k,k'}=F_{k,-k'}$.

We want to show that for matrices with this symmetry, in the continuous limit there is only one discrete eigenvalue. Note that this is not the correct symmetry for any TDDFT coupling matrices; we only want to provide a simple example to show that the symmetry of the coupling matrix for adiabatic TDDFT is important in determining the number of bound excitons.

The $\Omega^{(0)}+F$ matrix is

$$\begin{pmatrix} \omega^{(0)}_n-\omega'+F_{n,n} & F_{n,n-1} & \cdots & F_{n,0} & \cdots & F_{n,n-1} & F_{n,n} \\ F_{n,n-1} & \omega^{(0)}_{n-1}-\omega'+F_{n-1,n-1} & \cdots & F_{n-1,0} & \cdots & F_{n-1,n-1} & F_{n,n-1} \\ \vdots & \vdots & \ddots & \vdots & & \vdots & \vdots \\ F_{n,0} & F_{n-1,0} & \cdots & \omega^{(0)}_0-\omega'+F_{0,0} & \cdots & F_{n-1,0} & F_{n,0} \\ \vdots & \vdots & & \vdots & \ddots & \vdots & \vdots \\ F_{n,n-1} & F_{n-1,n-1} & \cdots & F_{n-1,0} & \cdots & \omega^{(0)}_{n-1}-\omega'+F_{n-1,n-1} & F_{n,n-1} \\ F_{n,n} & F_{n,n-1} & \cdots & F_{n,0} & \cdots & F_{n,n-1} & \omega^{(0)}_n-\omega'+F_{n,n} \end{pmatrix}. \tag{1}$$

The Jacobi rotation $M'$ for a matrix $M$ is defined by

$$M'=R^T_{i,j}(\theta)MR_{i,j}(\theta), \tag{2}$$

where $R_{i,j}(\theta)$ is a rotation matrix of dimension $(2n+1)\times(2n+1)$ that only acts on the $i$th row and the $j$th column:

$$R_{i,j}(\theta)=\begin{pmatrix} 1 & & & & & \\ & \ddots & & & & \\ & & r_{ii} & & r_{ij} & \\ & & & \ddots & & \\ & & r_{ji} & & r_{jj} & \\ & & & & & \ddots \\ & & & & & & 1 \end{pmatrix}. \tag{3}$$

Here, all matrix elements along the diagonal are 1 except $r_{ii}$ and $r_{jj}$, and all off-diagonal elements are zero except $r_{ij}$ and $r_{ji}$, and we have $r_{ii}=\cos\theta$, $r_{ij}=\sin\theta$, $r_{ji}=-\sin\theta$, $r_{jj}=\cos\theta$. Jacobi rotation of a matrix does not alter its eigenvalues.

We perform a series of Jacobi rotations of angle $\pi/4$ on $\Omega^{(0)}+F$:

$$\Omega=R^T_{n,n}R^T_{n-1,n-1}\cdots R^T_{1,1}\left(\Omega^{(0)}+F\right)R_{1,1}\cdots R_{n-1,n-1}R_{n,n}. \tag{4}$$

Due to the symmetry of $\Omega^{(0)}+F$, the resulting matrix $\Omega$ becomes block diagonal:

$$\Omega = \begin{pmatrix} \omega_n^{(0)} & & & & & & \\ & \omega_{n-1}^{(0)} & & & & & \\ & & \ddots & & & & \\ & & & \omega_0^{(0)}+F_{0,0} & \cdots & \sqrt{2}F_{n-1,0} & \sqrt{2}F_{n,0} \\ & & & \vdots & \ddots & \vdots & \vdots \\ & & & \sqrt{2}F_{n-1,0} & \cdots & \omega_{n-1}^{(0)}+2F_{n-1,n-1} & 2F_{n,n-1} \\ & & & \sqrt{2}F_{n,0} & \cdots & 2F_{n,n-1} & \omega_n^{(0)}+2F_{n,n} \end{pmatrix}. \tag{5}$$

Thus, $n$ of the eigenvalues of $\Omega$ are immediately given by $\omega_k^{(0)}$, $k=1,\dots n$. The remaining $n+1$ eigenvalues of $\Omega^{(0)}+F$ are obtained by diagonalizing an $(n+1)\times(n+1)$ submatrix.

The lower right $(n+1)\times(n+1)$ submatrix (denoted as $\tilde{\Omega}$) of $\Omega$ can be written as

$$\begin{aligned} \tilde{\Omega} &= \begin{pmatrix} \omega_0^{(0)} & \cdots & 0 & 0 \\ \vdots & \ddots & \vdots & \vdots \\ 0 & \cdots & \omega_{n-1}^{(0)} & 0 \\ 0 & \cdots & 0 & \omega_n^{(0)} \end{pmatrix} + \begin{pmatrix} F_{0,0} & \cdots & \sqrt{2}F_{n-1,0} & \sqrt{2}F_{n,0} \\ \vdots & \ddots & \vdots & \vdots \\ \sqrt{2}F_{n-1,0} & \cdots & 2F_{n-1,n-1} & 2F_{n,n-1} \\ \sqrt{2}F_{n,0} & \cdots & 2F_{n,n-1} & 2F_{n,n} \end{pmatrix} \\ &\equiv H^{(0)} + H^{(1)} \end{aligned} \tag{6}$$

Assuming we can apply perturbation theory by considering $H^{(0)}$ and $H^{(1)}$ as corresponding zeroth order and first order Hamiltonian, the eigenvalues of $\tilde{\Omega}$ up to second order are

$$\begin{aligned} \tilde{\omega}_0^{(2)} &= \omega_0^{(0)} + F_{0,0} + 2\sum_{m\neq 0} \frac{|F_{m,0}|^2}{\omega_0^{(0)}-\omega_m^{(0)}}, \\ \tilde{\omega}_{l\neq 0}^{(2)} &= \omega_l^{(0)} + 2F_{l,l} + 2\frac{|F_{l,0}|^2}{\omega_l^{(0)}-\omega_0^{(0)}} + 4\sum_{\substack{m\neq l\\ m\neq 0}} \frac{|F_{m,l}|^2}{\omega_l^{(0)}-\omega_m^{(0)}}. \end{aligned} \tag{7}$$

In the process of taking the continuous limit $n\to\infty$, neighboring matrix elements of $H^{(0)}$ and $H^{(1)}$ approach each other more and more closely. The differences between two eigenvalues of $\tilde{\Omega}$ to the second order then become

$$\begin{aligned} \tilde{\omega}_1^{(2)} - \tilde{\omega}_0^{(2)} &= \omega_1^{(0)} - \omega_0^{(0)} + 2(F_{1,1}-F_{0,0}) + F_{0,0} + 2\left[\sum_{m\neq 1} \frac{|F_{m,1}|^2}{\omega_1^{(0)}-\omega_m^{(0)}} - \sum_{m\neq 0} \frac{|F_{m,0}|^2}{\omega_0^{(0)}-\omega_m^{(0)}}\right] + 2\sum_{\substack{m\neq 1\\ m\neq 0}} \frac{|F_{m,1}|^2}{\omega_1^{(0)}-\omega_m^{(0)}} \\ &\overset{n\to\infty}{\to} F_{0,0} + 2\sum_{\substack{m\neq 1\\ m\neq 0}} \frac{|F_{m,1}|^2}{\omega_1^{(0)}-\omega_m^{(0)}} \neq 0, \\ \tilde{\omega}_{l+1}^{(2)} - \tilde{\omega}_l^{(2)} &= \omega_{l+1}^{(0)} - \omega_l^{(0)} + 2(F_{l+1,l+1}-F_{l,l}) + 4\left[\sum_{m\neq l+1} \frac{|F_{m,l+1}|^2}{\omega_{l+1}^{(0)}-\omega_m^{(0)}} - \sum_{m\neq l} \frac{|F_{m,l}|^2}{\omega_l^{(0)}-\omega_m^{(0)}}\right] + 2\left[\frac{|F_{l+1,0}|^2}{\omega_{l+1}^{(0)}-\omega_0^{(0)}} - \frac{|F_{l,0}|^2}{\omega_l^{(0)}-\omega_0^{(0)}}\right] \\ &\overset{n\to\infty}{\to} 0. \qquad (l\neq 0) \end{aligned} \tag{8}$$

Equation (8) shows that if $F$ is small compared to $\Omega$ so that it can be viewed as a perturbation, there will be at most one discontinuity in the eigenvalue spectrum of $\Omega^{(0)}+F$ in the continuous limit.

Here we use the matrix $F$ with the specified symmetry for the ease of demonstration, but the symmetry of matrix $F$ can actually be relaxed. A similar analysis can be applied to a real matrix $F$ that has $F_{k,k'} = F_{-k',-k} = F_{k',k}$.

## II. PROOF OF ONLY ONE BOUND EXCITON FOR SEPARABLE KERNELS

For separable adiabatic xc kernels $F^{(vc)(vc)}_{\mathbf{k},\mathbf{k}'} = A(\mathbf{k})B(\mathbf{q})$, $k$ and $k'$ are completely decoupled in the xc kernel. The symmetry $F^{(vc)(vc)}_{k,k'} = F^{(vc)(vc)}_{-k',-k} = F^{(vc)(vc)*}_{k',k}$ implies that such separable kernels can only have the form

$$F_{k,k'} = \pm A(k)A^*(k'). \tag{9}$$

The TDDFT excitation frequencies for the two-bands model with an adiabatic kernel are solved by

$$\sum_{\mathbf{k}'} \left[\omega^{cv}_{\mathbf{k}'}\delta_{\mathbf{k},\mathbf{k}'} + F^{(vc)(vc)}_{\mathrm{HXC},\mathbf{k},\mathbf{k}'}\right] \rho^{cv}_{\mathbf{k}'}(\omega) = \omega\rho^{cv}_{\mathbf{k}}(\omega). \tag{10}$$

For most 3D applications, the local-field effects can be left out. Since the Hartree kernel only contributes to the spectrum through the local-field effects, it can be neglected in Eq. (10). Consider an excitation below the band gap with frequency $\omega$:

$$(\omega - \omega_{\mathbf{k}})\rho^{cv}_{\mathbf{k}}(\omega) = \int_{\mathrm{FBZ}} \mathrm{d}\mathbf{k}'\; F^{(vc)(vc)}_{\mathbf{k},\mathbf{k}'}\rho_{\mathbf{k}'}(\omega) = \pm A(\mathbf{k}) \int_{\mathrm{FBZ}} \mathrm{d}\mathbf{k}'\; A^*(\mathbf{k}')\rho^{cv}_{\mathbf{k}'}(\omega) \equiv \pm A(\mathbf{k})C. \tag{11}$$

We therefore have

$$\rho^{cv}_{\mathbf{k}}(\omega) = \pm\frac{A(\mathbf{k})C}{\omega - \omega_{\mathbf{k}}}. \tag{12}$$

Multiply both sides with $A^*(\mathbf{k})$, and integrate over $\mathbf{k}$:

$$\int_{\mathrm{FBZ}} \mathrm{d}\mathbf{k}\; A^*(\mathbf{k})\rho^{cv}_{\mathbf{k}}(\omega) = C = \pm\int_{\mathrm{FBZ}} \mathrm{d}\mathbf{k}\; \frac{|A(\mathbf{k})|^2\, C}{\omega - \omega_{\mathbf{k}}}\;. \tag{13}$$

Thus,

$$1 = \pm\int_{\mathrm{FBZ}} \mathrm{d}\mathbf{k}\; \frac{|A(\mathbf{k})|^2}{\omega - \omega_{\mathbf{k}}}\;. \tag{14}$$

Since the excitation is below the band gap, $\omega - \omega_{\mathbf{k}} < 0$, and

$$1 = -\int_{\mathrm{FBZ}} \mathrm{d}\mathbf{k}\; \frac{|A(\mathbf{k})|^2}{\omega - \omega_{\mathbf{k}}}, \tag{15}$$

only a minus sign allows such an excitation. To show that there is at most one bound exciton for separable kernels, take the derivative of the right-hand side of Eq. (15) with respect to $\omega$:

$$\frac{\partial}{\partial\omega}\left[-\int_{\mathrm{FBZ}} \mathrm{d}\mathbf{k}\; \frac{|A(\mathbf{k})|^2}{\omega - \omega_{\mathbf{k}}}\right] = 2\int_{\mathrm{FBZ}} \mathrm{d}\mathbf{k}\; \frac{|A(\mathbf{k})|^2}{(\omega - \omega_{\mathbf{k}})^2} \geq 0. \tag{16}$$

Therefore, the right-hand side of Eq. (15) is monotonically increasing, and Eq. (15) can have at most one solution. This solution corresponds to a bound exciton.
